# Supplementary material for: Tree-Values: selective inference for regression trees
Source: arXiv:2106.07816 source file (2022-10-17)
Supplement: Supplementary file 1 [file appendix-varest-sims.tex]

\section{Simulations with Estimated Variance}
\label{appendix:varest_sims}

\textcolor{red}{Estimated variance sims. }
\textcolor{green}{Note-- if we can get this to fit in the main text then it might not need to be an appendix. }
